# Supplementary material for: Improved Regret for Differentially Private Exploration in Linear MDP
Source: arXiv:2202.01292 source file (2022-06-22)
Supplement: Supplementary file 1 [file appendix_switching_cost.tex]

\section{Analysis for switching cost}
\label{sec:switching-cost-appendix}
In our algorithm, we want to ensure that the policy is updated infrequently. The analysis of this switching cost follows in two steps: first we show that the potential function is upper bounded by $O(d \log K)$, then we show that the potential function increases by a constant whenever the policy updates. 

\begin{lemma} Let $\phi_i$ are $d-$dimensional vectors satisfying $\nn{\phi_i} \leq 1$. Let $A = \sum_{i=1}^K \phi_i \phi_i^\top + M_i + \lambda \I  + \lambtil \I$. Then, we have
\begin{equation*}
    \log \det A = O(d \log K)
\end{equation*}
\label{lem:L1-switchingcost}
\end{lemma}

\begin{proof}
Assume $\phi_i^d = (\alpha_1, \alpha_2, \dots, \alpha_d)^\top$. Since $\nn{\phi} \leq 1$, we have $|\alpha_i| \leq 1$ for all $i \in [d]$. Since $\phi_i^d (\phi_i^d)^\top = (\alpha_i \alpha_j)_{ij}$, the absolute value of each component of $\phi_i^d (\phi_i^d)^\top$ is no more than $1$. Hence, the absolute value of each component of $A_d$ is no more than $K + \lambda + \lambtil$. \dncomment{not true}

Use $\tilde{A}_d = (a_{ij})$ to denote a $d-$dimensional matrix satisfying the features above, i.e. $|a_{ij}| \leq K + \lambda + \lambtil$. Clearly, if the $1$st row and $j_\text{th}$ column are deleted, the rest $(d-1)$-dimensional matrix is $\tilde{A}_{d-1}$. Hence, we have:
\begin{align*}
    |\det(A_d)| &\leq \sum_{j=1}^d |a_{1d}| \cdot |\det(A_{d-1})|\\
    &\leq d \cdot (K + \lambda + \lambtil) \cdot |\det(A_{d-1})|\\
    &\leq d^d (K + \lambda + \lambtil)^d
\end{align*}
Hence, we have $\log \det A_d = d \log d + d\log(K + \lambda + \lambtil) = O(d \log K)$
\end{proof}

\begin{lemma}
Assume $m \leq n$, $A = \sum_{i=1}^m \phi_i \phi_i^\top + \M_i + \lambda \I + \lambtil \I$, $B = \sum_{i=1}^n \phi_i \phi_i^\top + \M_i + \lambda \I  + \lambtil \I$. Then, if $A^{-1} \npreceq 2B^{-1}$, we have
\begin{equation*}
    \log \det B \geq \log \det A + \log 2
\end{equation*}
\label{lem:L2-switchingcost}
\end{lemma}

First, we state the following two linear algebra facts that will be used in the proof:
\begin{fact}[Woodbury matrix identity] For any PSD matrices $A$, $\Delta \in \mathbb{R}^{d \times d}$. Suppose $A$ is invertible, then we have:
\begin{align*}
    (A + \Delta)^{-1} = A^{-1} - A^{-1} \Delta^{1/2}(\I + \Delta^{1/2} + A^{-1} \Delta^{1/2})^{-1} \Delta^{1/2} A^{-1}
\end{align*}
\end{fact}
\begin{fact}[Matrix determinant lemma] For any PSD matrices $A$, $\Delta \in \mathbb{R}^{d\times d}$, suppose $A$ is invertible, then 
\begin{equation*}
    \det(A + \Delta) = \det(\I + \Delta^{1/2} A^{-1} \Delta^{1/2}) \cdot \det(A)
\end{equation*}
\end{fact}

\begin{proof}
By the matrix determinant lemma, we only need to show that:
\begin{equation*}
    \lambda_{\max}(\I + \Delta^{1/2} A^{-1} \Delta^{1/2}) \geq 2
\end{equation*}
Since $A^{-1} \npreceq 2B^{-1}$, it must be the case that, for some $x$ with $\nn{x}_2 = 1$, and 
\begin{equation*}
    x^\top (A^{-1} -2B^{-1})x \geq 0 
\end{equation*}
Denote $\Delta = B - A \succ 0$. By Woodbury identity, we have:
\begin{align*}
    &\quad x^\top (A^{-1} - 2B^{-1})x \\
    &= x^\top (2 A^{-1} \Delta^{1/2}(\I + \Delta^{1/2} A^{-1} \Delta^{1/2})^{-1} \Delta^{1/2} A^{-1} - A^{-1})x\\
    &\geq 0
\end{align*}
Let $y = A^{-1/2}x$, we then have,
\begin{align*}
    &\quad 2y^\top A^{-1/2} \Delta^{1/2} (\I + \Delta^{1/2} A^{-1} \Delta^{1/2})^{-1} \Delta^{1/2} A^{-1/2} y\\
    &\geq \nn{y}_2^2
\end{align*}
Hence, 
\begin{equation*}
    \lambda_{\max} (A^{-1/2} \Delta^{1/2} (\I + \Delta^{1/2} A^{-1} \Delta^{1/2})^{-1} \Delta^{1/2} A^{-1/2}) \geq 1/2
\end{equation*}
Let us denote $H = A^{-1/2}\Delta^{1/2}$, we have:
\begin{equation*}
    \lambda_{\max} (H (\I + H^\top H)^{-1} H^\top) \geq 1/2
\end{equation*}
Let $H = U \Sigma V^\top$ be the SVD decomposition of $M$, where $U$ and $V$ are orthogonal and $\Sigma$ is diagonal. Then we have,
\begin{align*}
    &\quad H(\I + H^\top H )^{-1} H^\top\\
    &= U \Sigma V^\top (\I + V \Sigma^2 V^\top)^{-1} V \Sigma U^\top\\
    &= U \Sigma (\I + \Sigma^2)^{-1} \Sigma U^\top
\end{align*}
Note that $\Sigma = \mathrm{diag}(\sigma_1, \sigma_2, \dots, \sigma_d)$ is diagonal, we have
\begin{equation*}
    \max_i \frac{\sigma_i^2}{1 + \sigma_i^2} \geq 1/2 \Rightarrow \max_i \sigma_i^2 \geq 1
\end{equation*}
we additionally write $\I + \Delta^{1/2} A^{-1} \Delta^{1/2}$ as 
\begin{equation*}
    \I + \Delta^{1/2} A^{-1} \Delta^{1/2} = \I + H^\top H = \I + V \Sigma^2 V^\top
\end{equation*}
Thus we have
\begin{equation*}
    \lambda_{\max}(\I + \Delta^{1/2} A^{-1} \Delta^{1/2}) \geq 2
\end{equation*}
as desired. 
\end{proof}

Combining the lemmas above, we can now prove the switching cost bound in \Cref{thm:switchingcost}
\begin{proof}
Let $\{ k_1, k_2, \dots, k_{N_\text{switch}^\text{gl}} \}$ denote the update episodes $\tilde{k}$ from \Cref{alg:privrl}. By 
\Cref{lem:L2-switchingcost} we know $\det \Lambtil_{k_{i+1}} \geq 2 \det \Lambtil_{k_i} \geq 2^{k_{i+1}}\det \Lambtil_0$. Hence, by combining \Cref{lem:L1-switchingcost} we have $N_\text{switch}^\text{gl} \geq c_0 \log \det \Lambtil_K = O(d \log K)$
\end{proof}
