# Supplementary material for: Improved Regret for Differentially Private Exploration in Linear MDP
Source: arXiv:2202.01292 source file (2022-06-22)
Supplement: Supplementary file 2 [file DP.tex]

\section{Differential Privacy}

%%%%%%%%%%%%%%%%%%%%%%%%%%%%%%
% \begin{definition}[$\ell_2$-Sensitivity]
% Suppose we have a function $f: U  \rightarrow \mathbb{R}^d$.
% %
% Let $U,U'$ be two $t$-neighboring user sequences. Then the $\ell_2$-sensitivity is 
% \begin{align*}
%  \Delta_{f}  =  \| f(U) - f(U')\|_2 
% \end{align*}
% \end{definition}

\begin{definition}[Neighboring datasets]
We say that two datasets $x,y \in \mathbb{N}^n$ are neighboring (denoted by $x \sim y$) if $\|x-y\| =1$. 
\end{definition}

% The sensitivity of a mechanism refers to how much the output changes if the dataset changes by a small amount, here is the formal definition:
% %%%%%%%%%%%%%%%%%%%%%%%
% %% Def
% %%%%%%%%%%%%%%%%%%%%%%%
% \begin{definition}[$\ell_2 $ sensitivity]
% Let $f:\mathbb{N}^n\rightarrow \mathbb{R}^d$ be an arbitrary function. The  $\ell_2$ sensitivity of $f$ is given by $\Delta_2(f) = \max_{x,y}\|f(x) - f(y)\|_2$.
% \end{definition}

%%%%%%%%%%%%%%%%%%%%%%%
%% Def
%%%%%%%%%%%%%%%%%%%%%%%
\begin{definition}[Renyi divergence] Let $P$ and $Q$ be distributions on $\Sigma$. For all $\alpha\in (1,\infty)$ we define Renyi divergence of order $\alpha$ between $P$ and $Q$ as 
\begin{align*}
    D_\alpha(P \parallel Q) = \frac{1}{\alpha-1} \log\pp{\int_{\Sigma}  P(x)^\alpha Q(x)^{\alpha-1} } 
\end{align*}
\end{definition}

%%%%%%%%%%%%%%%%%%%%%%%
%% Def
%%%%%%%%%%%%%%%%%%%%%%%
\begin{definition}[Gaussian Noise Matrix]\label{def:GNM}
We define a Gaussian Noise Matrix as $\Z$, where $\Z$ is a $d\times d$ matrix and each coordinate of $\Z$ is sampled from the Gaussian distribution $\Z_{i,j} \sim \cN(0, \sigma^2)$. We use concentration bounds found in \cite{shariff2018differentially} and \cite{tao2012topics} to bound the norm $\|\Z\|_2$ with high probability, that is for any $\beta'$ we have:
\begin{align}
\label{eq:GauNormBound}
    \pr{\|\Z\|_2 > \sigma \pp{4\sqrt{d + 1} + 2\ln(1/\beta')}} \leq \beta'
\end{align}
\end{definition}

Next we define the Gaussian mechanism. 

%%%%%%%%%%%%%%%%%%%%%%%
%% Def
%%%%%%%%%%%%%%%%%%%%%%%
\begin{definition}[Gaussian Mechanism]
\label{lem:gaubound}
% Given a function $f:\mathbb{N}^n\rightarrow \mathbb{R}^d$ and an input dataset $x$.
% The Gaussian mechanism with parameter $\sigma$ adds noise from $\mathcal{N}(0, \sigma^2)$ to each component of $f(x)$.
Let $q:\cX^n \rightarrow \mathbb{R}$ be a sensitivity $\Delta$ query. For any input $X\in \cX^n$, the Gaussian mechanism is given by $\cM_G(x) = q(x) + \cN\pp{0, \frac{\Delta^2}{2\rho}}$.
Then $\cM_G$ satisfies ${\rho}$-zCDP and is 
$\pp{\sqrt{\frac{\Delta}{\rho}\ln(2/\beta)}, \beta}$-accurate.
\end{definition}

%%%%%%%%%%%%%%%%%%%%%%%
%% 
%%%%%%%%%%%%%%%%%%%%%%%

%%%%%%%%%%%%%%%%%%%%%%%
%% Def
%%%%%%%%%%%%%%%%%%%%%%%
\begin{definition} ($k$-neighboring user sequences)
Given two T users sequences $U$ and $U'$ given by $U = (u_1, u_2, \dots, u_T)$ and $U' = (u'_1, u'_2, \dots, u'_T)$. We say $U$ and $U'$ are t-neighboring user sequences if they only differ in their t-th user. Formally, we have
\begin{align*}
    u_i = u'_i \tag{$\forall i \in [1, T], i \neq t$}\\
    u_t \neq u'_t
\end{align*}
\end{definition}

\begin{lemma}[Gaussian Matrix Mechanism]
Suppose we have a dataset $X =\{ \x_1, \ldots, \x_n\}$, where each $\x_i\in \mathbb{R}^d$ is a $d$-dimensional vector with bounded $\ell_2$-norm such that: $\|\x_i\|_2\leq L$ for all $i\in [n]$. 
Consider releasing the following statistic privately: $\V = \sum_{i=1}^n \x_i\x_i^\top$, where each $\x_i\x_i^\top$ alters the Frobenius norm by at most $L^2$.
The Gaussian Matrix Mechanism samples the noise matrix $\Z'$, where $\Z'\in\mathbb{R}^{d\times d}$ is a random matrix where each entry $\Z'_{i,j} \sim  \cN\pp{0, \frac{L^4}{2\rho}}$ i.i.d, gets the symmetric matrix $\Z = (\Z' + {\Z'}^{\top})/\sqrt{2}$ and outputs:
\begin{align*}
    \cM_G(X) = \sum_{i=1}^n \x_i\x_i^\top + \Z
\end{align*}
Then $\cM_G$ satisfies ${\rho}$-zCDP and is $\pp{\frac{L^2\pp{4\sqrt{d+1} + 2\ln(2/\beta)}}{\sqrt{2\rho}}, \beta}$-$\ell_2$-accurate.
% $\pp{L^2\sqrt{\frac{}{2\rho}} \pp{4\sqrt{d+1} + 2\ln(2/\beta)}, \beta}$-$\ell_2$-accurate.
\end{lemma}

\begin{definition}[$\ell_2$-Sensitivity]
Suppose we have a function $f: U  \rightarrow \mathbb{R}^d$.
Let $U,U'$ be two $t$-neighboring user sequences. Then the $\ell_2$-sensitivity is 
\begin{align*}
 \Delta_{f}  =  \| f(U) - f(U')\|_2 
\end{align*}
\end{definition}

% \newpage
\paragraph{Private Counters: } We use the binary mechanism from \cite{chan2011private}. The framework consists of representing any stream of statistics as the sum of a number of $p$-sums. Each $p$-sum is released using differential privacy and then aggregated. Note that each $p$-sum is a query with sensitivity $1$.

First we describe two simple mechanisms: To set up the context, suppose that over $T$ rounds,  we observe a stream $s_1, \ldots, s_T$. The first algorithm consists of releasing a partial count with just one $p$-sum on every round, that is the algorithm adds Gaussian noise satisfying $\rho'$-zCDP to every partial sum: On each round $t\leq T$ this mechanism releases the partial sum up to round $t$ with Gaussian noise: $\sum_{i=1}^t s_i + \Gau\pp{\tfrac{1}{2\rho'}}$. 
Then this mechanism satisfies $(T\rho')$-zCDP. If we set $\rho' = \frac{\rho}{T}$, then the mechanism satisfies $\rho$-zCDP and the accuracy is $O(\sqrt{\frac{T}{\rho}\ln(2/\beta)})$.

The second algorithm releases $t$ p-sums on each round $t$. Let $\tilde{\sigma}^t = s_{t} +  z_t$, where $z_t\sim\Gau\pp{\tfrac{1}{2\rho}}$ then release $\tilde{S}_t = \sum_{i=1}^t \tilde{\sigma}^i$. Note that each item appears in at most $1$ $p$-sum thus it satisfies $\rho$-zCDP and 
$S_t- \tilde{S}_t = \sum_{i=1}^t z_i$. 
Therefore, from \cref{lem:gaubound} the algorithm is  $(\sqrt{\frac{T \ln(2/\beta)}{\rho}}, \beta)$-accurate.

% 1) Write BM with zCDP.
\paragraph{Binary Gaussian Mechanism} 
Represent the $\sigma_{1}^t, \ldots, \sigma_{m}^t$ the partial sums of the binary mechanism on round $t$, such that $S_t = \sum_{i=1}^t s_i = \sum_{j=1}^m \sigma_{ j}^t$. The binary mechanism uses the following informal observation:
\begin{observation}[\cite{chan2011private}]\label{ob:binary}
 Suppose that each item in the stream appears in $x$  $p$-sums and there are at most $y$ $p$-sums, if we add Gaussian noise with parameter $\frac{x}{2\rho}$ to the $y$ $p$-sums such that each it satisfies $\frac{\rho}{x}$-zCDP then the mechanism satisfies $\rho$-zCDP. The high probability error of each partial sum is at most $O\pp{\sqrt{\frac{xy}{\rho}\log\pp{2/\beta}}}$.
\end{observation}

The Binary Mechanism can represent each sum $S_t$ with $m=\log(T)$ partial sums on each round. Since each item $s_i$ in the stream will appear in at most $\log(T)$ partial sums we have to add Gaussian noise with parameter $\log(T)/\rho$ to satisfy $\rho$-zCDP. Let $\tilde{\sigma}^t_i$ be a noisy partial sum defined by $\tilde{\sigma}^t_i = \sigma^t_i + z^t_i$
where $z^t_i \sim  \cN\pp{0,\frac{\log(T)}{2\rho}}$.
Each round $t$, the binary mechanism releases $\tilde{S}_t = \sum_{i=1}^m \tilde{\sigma}_i$.
The error $|\tilde{S}_t - S_t|$ is the sum of $\log(T)$ Gaussian random variables with parameter $\log(T)/\rho$, therefore the bound from \cref{lem:gaubound} gives that the binary mechanism is $\pp{\sqrt{\log(T)^2\log(2/\beta) /\rho }, \beta}$-accurate.

In this paper we define the Gaussian Noise Matrix $\Z \in \mathbb{R}^d\times \mathbb{R}^d$, where each coordinate is sampled i.i.d from the Gaussian distribution with parameter $\sigma$.

In this paper we observe a sequence of vectors $\x_1,\ldots,\x_T$ where each $\x_i$ represents the data of one person. Furthermore, 
we assume that data vector has bounded $\ell_2$ norm  $\|\x_i\|_2 \leq L$.

Finally, 
\begin{lemma}[Gaussian Binary Matrix Mechanism (GBMM)]
\gv{GV: Will remove or update this. }
Let $\cC$ be a binary mechanism private counter initialized with parameter $\rho$.

The GBMM takes as input a stream of $d$-dimensional vectors $ \x_1, \ldots, \x_K$ over a sequence of $K$ episodes.

On each episode $k\in [K]$, the goal is to release the following statistic $\V_k = \sum_{i=1}^k \x_i\x_i^\top$. Note that $\|\x_i\x_i^\top\|_2\leq L^2$.
On episode $k$, the GBMM releases $\V_k + \mH_k$, where $\mH_k$ is the sum of at most $\log(T=HK)$ Gaussian noise matrices with parameter $\log(K)L^4/\rho$.
Then, GBMM satisfies $\rho$-zCDP and  $\| \mH_k \|_2 \leq \frac{L^2\log(K) \pp{4\sqrt{d+1} + 2\ln(2/\beta)} }{\sqrt{2\rho}}$
\end{lemma}

\swcomment{can we not use $\x$? is this supposed to be a general result or specificially for our algo?}

% \begin{lemma}[Gaussian Binary Matrix Mechanism (GBMM)]
% Suppose we observe a stream of $d$-dimensional vectors $ \x_1, \ldots, \x_K$ over a sequence of $K$ episodes.Each $\x_i\in \mathbb{R}^d$ has bounded $\ell_2$-norm such that: $\|\x_i\|_2\leq L$ for all $i\in [n]$. On each episode $k\in [K]$, the goal is to release the following statistic $\V_k = \sum_{i=1}^k \x_i\x_i^\top$. Note that $\|\x_i\x_i^\top\|_2\leq L^2$.
% %
% On episode $k$, the GBMM releases $\V_k + \mH_k$, where $\mH_k$ is the sum of at most $\log(T=K)$ Gaussian noise matrices with parameter $\log(K)L^4/\rho$.
% Then, GBMM satisfies $\rho$-zCDP and  $\| \mH_k \|_2 \leq \frac{L^2\log(K) \pp{4\sqrt{d+1} + 2\ln(2/\beta)} }{\sqrt{2\rho}}$
% \end{lemma}

% Each $\tilde{\sigma_i}$ satisfies $\frac{\rho}{\log(T)}$-zCDP so releasing  the sequence $\tilde{S}_1,\ldots,\tilde{S}_T$ satisfies $\rho$-zCDP.
% to each $\sigma_i$ so that $$ satisfies $\frac{\rho}{\log(T)}$-zCDP guarantees that releasing the sequence satisfies $\rho$-zCDP.

% \begin{algorithm}[H]
% \SetAlgoLined
  
% \caption{$\BM$}\label{alg:binMech}
% \end{algorithm}

%%%%%%%%%%%%%%%%%%%%%%%%%%%%%%%%%%%%%%%%%%%%%%%%%%
%%%%%%%%%%%%%%%%%%%%%%%%%%%%%%%%%%%%%%%%%%%%%%%%%%
\begin{definition}[Accuracy]
We say that a mechanism $\cM:\cX^*\rightarrow [0,1]$ is $(\alpha, \beta)$-accurate if with probability at least $1-\beta$ it has error at most $\alpha$.
\end{definition}

%%%%%%%%%%%%%%%%%%%%%%%%%%%%%%%%%%%%%%%%%%%%%%%%%%
%%%%%%%%%%%%%%%%%%%%%%%%%%%%%%%%%%%%%%%%%%%%%%%%%%
\begin{definition}[Matrix norm error]
We say that a mechanism $\cM:\cX^*\rightarrow [0,1]$ is $(\alpha, \beta)$-accurate if with probability at least $1-\beta$ it has $\ell_2$-error at most $\alpha$.
% The matrix mechanism is $(\alpha,\beta)$-accurate if $\|\sum_{i=1}^n \x\x^\top -  \cM_G(X) \|_2 \leq \alpha$ with probability at least $1-\beta$.
\end{definition}
