# Supplementary material for: Improved Regret for Differentially Private Exploration in Linear MDP
Source: arXiv:2202.01292 source file (2022-06-22)
Supplement: Supplementary file 3 [file math_background.tex]

\section{Math Background}

\begin{definition}[PSD]\label{def:psd}
A matrix $M\in\mathbb{R}^{d\times s}$ is positive semi-definite (denoted by $M\succ 0$ if for all $d\in\mathbb{R}^d$ we have $x^\top M \geq 0$. We say $M\succ N$ if $M-N\succ 0$.
\end{definition}

\begin{definition}\label{def:switchingcost}
For an algorithm that deploys policies $(\pi_1, \ldots, \pi_T)$ its global switching cost given by:
\begin{align*}
    \sum_{t=1}^T I(\pi_t \neq \pi_{t+1})
\end{align*}
\end{definition}

\begin{definition}(Vector and Matrix Norm)
For any symmetric positive-semidefinite matrix $\mathbb{M}$, we define a norm on vectors as followed: $\nn{\mathbf{x}}_{\mathbf{M}} = \sqrt{\mathbf{x}^\top \mathbf{M} \mathbf{x}}$. 

For a matrix $\mathbf{M}$, we use the following notations for norm of $\mathbf{M}$:
\begin{itemize}
    \item Operator norm: Given a vector norm $\nn{\cdot}$, we can define the corresponding operator norm as: 
    \begin{equation}
        \nn{\mathbf{M}} = \max_{\mathbf{x}: \nn{\mathbf{x}} = 1} \{\nn{\mathbf{Mx}}\}
    \end{equation}
    \item Spectral norm: A special case of the operator norm when we have L2 vector norm. The spectral norm of a matrix $\mathbf{M}$ is the largest singular value of $\mathbf{M}$: 
    \begin{equation}
        \nn{\mathbf{M}}_2 = \sigma_{\max} (\mathbf{M})
    \end{equation}
\end{itemize}
\end{definition}
